# Supplementary material for: Convective meta-thermal dispersion for self-adaptive cooling enhancement
Source: arXiv:2405.07161 source file (2024-05-12)
Supplement: Supplementary file 1 [file Supplementary_information.pdf]

# Convective meta-thermal dispersion for self-adaptive cooling enhancement

Xinchen Zhou[1,2], Ruzhu Wang[2], Xiaoping Ouyang[3,*], Jiping Huang[1,*]

[1]Department of Physics, State Key Laboratory of Surface Physics, Key Laboratory of Micro and Nano Photonic Structures (MOE), Fudan University, Shanghai 200438, China;
[2]School of Mechanical Engineering, Institute of Refrigeration and Cryogenics, Engineering Research Center of Solar Power and Refrigeration (MOE), Shanghai Jiao Tong University, Shanghai 200240, China;
[3]School of Materials Science and Engineering, Xiangtan University, Xiangtan 411105, China.

*To whom correspondence should be addressed; E-mail: oyxp2003@aliyun.com, jphuang@fudan.edu.cn.

**The file includes:**
Supplementary Notes 1-5
Supplementary Figs. 1-8
Supplementary Tables 1-8
References

# Supplementary Notes

# 1 General theory for CMTD

For analysis purposes, we examine two extreme conditions: $\kappa_{\mathrm{t}} \to \infty$ and $\kappa_{\mathrm{t}} \to 0$ (both under $\kappa_{\mathrm{r}} \to \infty$), where "$\kappa_{\mathrm{t}} \to \infty$" denotes a structure with ultrahigh thermal conductivity ($\kappa_{\mathrm{A}} = \kappa_{\mathrm{B}} \to \infty$, without CMTD), while "$\kappa_{\mathrm{t}} \to 0$" represents a structure with alternating materials of ultrahigh and ultralow thermal conductivities ($\kappa_{\mathrm{A}} \to \infty$ and $\kappa_{\mathrm{B}} \to 0$, with CMTD), as depicted in Supplementary Fig. 1.

## 1.1 Scenario without CMTD

In the scenario of $\kappa_{\mathrm{t}} \to \infty$ (without CMTD, Supplementary Fig. 1a), $T_{\mathrm{f}}|_{\theta\to 0}$ approaches $T_{\mathrm{f}}|_{\theta=\pi}$ ($T_{\mathrm{f,out}}$) due to the highly efficient heat transfer along the tangential direction within the package region. We assume a uniform temperature distribution on the outer surface of the package structure and the fluid in the channel along the tangential direction. This uniformity implies that the heat flow from the IHS to the fluid is independent of the tangential direction $\theta$. Following energy conservation, Newton's cooling equation, and heat flux under a cylindrical coordinate system, the heat flux on the outer surface of the package structure $q_2$ is given by:

$$q_2 = \begin{cases} \dfrac{\pi R_1^2 \dot{\phi}_{\mathrm{h}}}{2\pi R_2} \\ h\left(T_2 - T_{\mathrm{f,out}}\right) \\ \dfrac{\kappa_{\mathrm{r}}}{R_2}\dfrac{T_1 - T_2}{\ln\left(R_2/R_1\right)} \end{cases}, \tag{S1}$$

where $T_1$ and $T_2$ are the temperatures of the inner and outer surfaces of the package structure, respectively. From this equation, we obtain the relationship between $T_1$ and $T_{\mathrm{f,out}}$

$$T_1 = \frac{R_1^2 \dot{\phi}_{\mathrm{h}}}{2\kappa_{\mathrm{r}}} \ln\frac{R_2}{R_1} + \frac{R_1^2 \dot{\phi}_{\mathrm{h}}}{2hR_2} + T_{\mathrm{f,out}}. \tag{S2}$$

The temperature distribution in the IHS is given by

$$T = \frac{1}{4}\frac{\dot{\phi}_{\mathrm{h}}}{\kappa_{\mathrm{h}}}\left(R_1^2 - R^2\right) + T_1,\ R \in [0, R_1]. \tag{S3}$$

Substituting Eq. (S3) into Eq. (S4) and considering

$$T_{\mathrm{f,out}} = T_{\mathrm{f,in}} + \frac{\pi R_1^2 \dot{\phi}_{\mathrm{h}} d_{\mathrm{z}}}{c\dot{m}}, \tag{S4}$$

where $\dot{m}$ is the mass flow of the working fluids, we get the temperature distribution of IHS

$$T = \frac{1}{4}\frac{\dot{\phi}_{\mathrm{h}}}{\kappa_{\mathrm{h}}}\left(R_1^2 - R^2\right) + \frac{R_1^2 \dot{\phi}_{\mathrm{h}}}{2\kappa_{\mathrm{r}}} \ln\frac{R_2}{R_1} + \frac{R_1^2 \dot{\phi}_{\mathrm{h}}}{2hR_2} + T_{\mathrm{f,in}} + \frac{\pi R_1^2 \dot{\phi}_{\mathrm{h}} d_{\mathrm{z}}}{c\dot{m}},\ R \in [0, R_1]. \tag{S5}$$

Then we solve three typical temperatures of the IHS, the maximum, average, and minimum values, for ease of verification. The minimum value of the IHS occurs when $R = R_1$

$$T_{\mathrm{min}} = \frac{R_1^2\dot{\phi}_{\mathrm{h}}}{2\kappa_{\mathrm{r}}}\ln\frac{R_2}{R_1} + \frac{R_1^2\dot{\phi}_{\mathrm{h}}}{2hR_2} + T_{\mathrm{f,in}} + \frac{\pi R_1^2\dot{\phi}_{\mathrm{h}}d_{\mathrm{z}}}{c\dot{m}}. \tag{S6}$$

The maximum value of the IHS temperature occurs when $R = 0$

$$T_{\mathrm{max}} = \frac{1}{4}\frac{\dot{\phi}_{\mathrm{h}}}{\kappa_{\mathrm{h}}}R_1^2 + \frac{R_1^2\dot{\phi}_{\mathrm{h}}}{2\kappa_{\mathrm{r}}}\ln\frac{R_2}{R_1} + \frac{R_1^2\dot{\phi}_{\mathrm{h}}}{2hR_2} + T_{\mathrm{f,in}} + \frac{\pi R_1^2\dot{\phi}_{\mathrm{h}}d_{\mathrm{z}}}{c\dot{m}}. \tag{S7}$$

As $q$ is independent of $\theta$, the temperature distribution is also independent of $\theta$. We then obtain the average temperature of the IHS by

$$T_{\mathrm{ave}} = \frac{1}{R_1}\int_0^{R_1} T\mathrm{d}R. \tag{S8}$$

## 1.2 Scenario with CMTD

When $\kappa_{\mathrm{t}} \to 0$, the temperature distribution in the package structure along the tangential direction is different. Hence, when the heat capacity flow rate of the working fluid is low, the temperature distribution within the annular flow channel undergoes modifications. In contrast to the first scenario, we assume that as the fluid enters the annular flow channel, its temperature matches the inlet temperature ($T_{\mathrm{f}}|_{\theta=0} \to T_{\mathrm{f,in}}$). Moving along the flow direction, the temperature gradually increases. Consequently, the maximum temperature of the IHS shifts to the right by a distance of $a$. Establishing a sub-coordinate system with the highest temperature point as the center, we further assume that the heat flux within the IHS extends radially outward from the highest temperature point towards the package structure. In the sub-coordinate system, the temperature distribution in the IHS along the radial direction is

$$T = \frac{1}{4}\frac{\dot{\phi}_{\mathrm{h}}}{\kappa_{\mathrm{h}}}\left(r_1^2 - r^2\right) + T_1,\ r \in [0, r_1]\,. \tag{S9}$$

Acoording to the geometric relationship, $r_1$ is determined as

$$r_1 = \sqrt{R_1^2 + a^2 - 2aR_1\cos(\pi - \theta)}. \tag{S10}$$

Substituting Eq. (S10) into Eq. (S9), we get

$$T = \frac{1}{4}\frac{\dot{\phi}_{\mathrm{h}}}{\kappa_{\mathrm{h}}}\left[R_1^2 + a^2 - 2aR_1\cos(\pi - \theta) - r^2\right] + T_1,\ r \in [0, r_1]. \tag{S11}$$

The minimum temperature of the IHS exists at the position $\theta = 0$ and $r = r_1$. Combining Eqs. (S2) and (S11), we have

$$T_{\mathrm{min}} = \frac{R_1^2\dot{\phi}_{\mathrm{h}}}{2\kappa_{\mathrm{r}}}\ln\frac{R_2}{R_1} + \frac{R_1^2\dot{\phi}_{\mathrm{h}}}{2hR_2} + T_{\mathrm{f,in}}. \tag{S12}$$

The expression of the maximum temperature of the IHS is obtained when $\theta = 0$ (or $\theta = \pi$) and $r = 0$

$$\begin{aligned} T_{\max} &= \frac{1}{4}\frac{\dot{\phi}_{\rm h}}{\kappa_{\rm h}}\left(R_1 + a\right)^2 + \frac{R_1^2\dot{\phi}_{\rm h}}{2\kappa_{\rm r}}\ln\frac{R_2}{R_1} + \frac{R_1^2\dot{\phi}_{\rm h}}{2hR_2} + T_{\rm f,in} \\ &= \frac{1}{4}\frac{\dot{\phi}_{\rm h}}{\kappa_{\rm h}}\left(R_1 - a\right)^2 + \frac{R_1^2\dot{\phi}_{\rm h}}{2\kappa_{\rm r}}\ln\frac{R_2}{R_1} + \frac{R_1^2\dot{\phi}_{\rm h}}{2hR_2} + T_{\rm f,out}. \end{aligned} \tag{S13}$$

Solving Eq. (S13), we get

$$a = \frac{\pi R_1 \kappa_{\rm h} d_{\rm z}}{c\dot{m}}, \tag{S14}$$

$$T_{\max} = \frac{1}{4}\frac{\dot{\phi}_{\rm h}}{\kappa_{\rm h}}\left(R_1 + \frac{\pi R_1 \kappa_{\rm h} d_{\rm z}}{c\dot{m}}\right)^2 + \frac{R_1^2\dot{\phi}_{\rm h}}{2\kappa_{\rm r}}\ln\frac{R_2}{R_1} + \frac{R_1^2\dot{\phi}_{\rm h}}{2hR_2} + T_{\rm f,in}. \tag{S15}$$

Combining Eq. (S11) with Eq. (S15), we have

$$\begin{aligned} T_1 = &\frac{1}{4}\frac{\dot{\phi}_{\rm h}}{\kappa_{\rm h}}\left(R_1 + \frac{\pi R_1 \kappa_{\rm h} d_{\rm z}}{c\dot{m}}\right)^2 + \frac{R_1^2\dot{\phi}_{\rm h}}{2\kappa_{\rm r}}\ln\frac{R_2}{R_1} + \frac{R_1^2\dot{\phi}_{\rm h}}{2hR_2} + T_{\rm f,in} \\ &- \frac{1}{4}\frac{\dot{\phi}_{\rm h}}{\kappa_{\rm h}}\left[R_1^2 + a^2 - 2aR_1\cos(\pi - \theta)\right]. \end{aligned} \tag{S16}$$

Therefore, the temperature distribution in the IHS reads

$$T = \frac{1}{4}\frac{\dot{\phi}_{\rm h}}{\kappa_{\rm h}}\left[\left(R_1 + \frac{\pi R_1 \kappa_{\rm h} d_{\rm z}}{c\dot{m}}\right)^2 - r^2\right] + \frac{R_1^2\dot{\phi}_{\rm h}}{2\kappa_{\rm r}}\ln\frac{R_2}{R_1} + \frac{R_1^2\dot{\phi}_{\rm h}}{2hR_2} + T_{\rm f,in}, r \in [0, r_1]. \tag{S17}$$

Combining Eq. (S14) with Eq. (S17), and making an integral average

$$T_{\rm ave} = \frac{1}{2\int_0^{\pi} r_1 {\rm d}\theta} \cdot 2\int_0^{\pi}\int_0^{r_1} T{\rm d}r{\rm d}\theta, \tag{S18}$$

we obtain the average IHS temperature Eq. (1).

# 2 Analytical form of convective heat transfer coefficients

The convective heat transfer coefficient between the package structure and the cooling fluid, denoted as $h$, is governed by various parameters, and its specific expression is given by:

$$h = \frac{Nu \cdot \kappa_{\rm f}}{\mathscr{L}_{\rm c}}. \tag{S19}$$

Here, $Nu$ represents the Nusselt number, and $\mathscr{L}_{\rm c}$ denotes the characteristic length. The $Nu$ can be further expressed as:

$$Nu = \mathscr{C} Re^m Pr^n \tag{S20}$$

where $\mathscr{C}$ is a constant, $Re$ represents the Reynolds number ($Re = v_{\mathrm{f,in}}\mathscr{L}_{\mathrm{c}}\rho_{\mathrm{f}}/\mu$), and $Pr$ represents the Prandtl number ($Pr = c_{\mathrm{f}}\mu/\kappa_{\mathrm{f}}$). To fully define the formula for $h$, it is necessary to further specify the expression for $\mathscr{L}_{\mathrm{c}}$. According to the definition, $\mathscr{L}_{\mathrm{c}}$ can be written as:

$$\mathscr{L}_{\mathrm{c}} = 4\frac{A}{W} = 4\frac{(R_3 - R_2)dz}{2(R_3 - R_2 + d_{\mathrm{z}})} = 2\frac{R_3 - R_2}{(R_3 - R_2)/d_{\mathrm{z}} + 1}. \tag{S21}$$

Here, $A$ is the cross-sectional area of fluid flow, and $W$ is the wet perimeter of the fluid-immersed channel (Supplementary Fig. 2). Two-dimensional heat transfer models can be considered as a section extracted from a three-dimensional heat transfer model with infinite thickness, ensuring that their temperature distribution is not influenced by the boundaries. Therefore, $d_{\mathrm{z}}$ can be treated as infinite, leading to:

$$\mathscr{L}_{\mathrm{c}} = 2(R_3 - R_2). \tag{S22}$$

# 3 Acquisition of convective heat transfer correlations

Supplementary Note 2 indicates that determining $\mathscr{C}$, $m$, and $n$ is required to obtain the expression for $h$. Let us revisit the expression for $\mathrm{Nu}$ in Eq. (S20), where the technique for deriving convective heat transfer correlation in heat transfer is employed. We utilize this method through finite element simulation, focusing on the heat transfer model presented in Fig. 1e. By keeping $\mathrm{Re}$ constant, the expression for $\mathrm{Nu}$ can be expressed as:

$$\ln \mathrm{Nu} = \ln \mathscr{C}' + n \ln \mathrm{Pr}. \tag{S23}$$

By altering the specific heat capacity $c_{\mathrm{f}}$ of the fluid to change $\mathrm{Pr}$, $\mathrm{Nu}$ will consequently change. The slope of $\ln \mathrm{Nu}$ and $\ln \mathrm{Pr}$ provides the value of $n$ (Supplementary Fig. 5a, Supplementary Table 1). Similarly, the equation can be rewritten as:

$$\ln \frac{\mathrm{Nu}}{\mathrm{Pr}^n} = \ln \mathscr{C} + m \ln \mathrm{Re}. \tag{S24}$$

Maintaining $\mathrm{Pr}$ constant and varying $\mathrm{Re}$, and taking the slope of $\ln\left(\mathrm{Nu}/\mathrm{Pr}^m\right)$ and $\ln \mathrm{Re}$, allows us to determine $m$ and $\mathscr{C}$ (Supplementary Fig. 5b, Supplementary Table 2). Following this method, we obtain:

$$\mathrm{Nu} = 4.394\mathrm{Re}^{0.062}\mathrm{Pr}^{0.061} \tag{S25}$$

for the case without CMTD, and

$$\mathrm{Nu} = 5.105\mathrm{Re}^{0.035}\mathrm{Pr}^{0.033} \tag{S26}$$

for the case with CMTD.

It is evident that under the same structural and fluidic parameters, the convective heat transfer correlations for the cases with and without CMTD differ. This difference arises because the tangential local convective heat transfer coefficient is given by:

$$h_\theta = -\frac{\kappa_\mathrm{f}}{\Delta T_\theta}\left(\frac{\partial T}{\partial R}\right)_\theta\bigg|_{R=R_2}, \tag{S27}$$

where $h_\theta$ is the tangential local convective heat transfer coefficient and $\Delta T_\theta$ is the tangential temperature difference between the outer surface of the package structure and the cooling fluid. Therefore, the total heat transfer coefficient reads:

$$h_\mathrm{t} = \frac{\int_0^\pi h_\theta d\theta}{\pi}. \tag{S28}$$

By adjusting the heat flux inside the package region, the temperature distribution of the fluid inside the channel can be changed, affecting $h_\theta$ and ultimately the convective heat transfer correlation.

# 4 Calculations of the equivalent radial and tangential thermal conductivities of the package structure

## 4.1 Thermal resistance on the radial direction

In cylindrical coordinates, the steady-state heat conduction differential equation without the IHS is given by:

$$\frac{1}{R}\frac{\partial}{\partial R}\left(\kappa R\frac{\partial T}{\partial R}\right) + \frac{1}{R^2}\frac{\partial}{\partial \theta}\left(\kappa\frac{\partial T}{\partial \theta}\right) + \frac{\partial}{\partial z}\left(\kappa\frac{\partial T}{\partial z}\right) = 0. \tag{S29}$$

First, consider the case where heat flux propagates only radially, as shown in Supplementary Fig. 4a. For simplicity, assume the material has constant properties, hence:

$$\frac{\mathrm{d}}{\mathrm{d}R}\left(R\frac{\mathrm{d}T}{\mathrm{d}R}\right) = 0. \tag{S30}$$

Integrating this equation and setting:

$$\begin{cases} T = T_1, R = R_1 \\ T = T_2, R = R_2 \end{cases}. \tag{S31}$$

we obtain:

$$\frac{\mathrm{d}T}{\mathrm{d}R} = \frac{1}{R}\frac{T_2 - T_1}{\ln(R_2/R_1)}. \tag{S32}$$

According to Fourier's law, the radial heat flux is:

$$q_\mathrm{r} = -\kappa\frac{\mathrm{d}T}{\mathrm{d}R}. \tag{S33}$$

Substituting Eq. (S32) into Eq. (S33), we have:

$$q_\mathrm{r} = \frac{\kappa}{R}\frac{T_1 - T_2}{\ln(R_2/R_1)}. \tag{S34}$$

For discussion convenience, converting heat flux to heat flux, and defining the product of the circumference corresponding to the central angle $(\theta_2 - \theta_1)$ and the thickness $l$ of the ring as the heat transfer area:

$$Q_{\mathrm{r}} = (\theta_2 - \theta_1)\, Rlq_{\mathrm{r}} = \frac{(\theta_2 - \theta_1)\,\kappa l(T_1 - T_2)}{\ln(R_2/R_1)} = \frac{T_1 - T_2}{\ln(R_2/R_1)\big/\left[(\theta_2 - \theta_1)\,\kappa l\right]}. \tag{S35}$$

In this scenario, the thermal resistance is $\ln(R_2/R_1)\big/\left[(\theta_2 - \theta_1)\,\kappa l\right]$.

## 4.2 Thermal resistance on the tangential direction

We then consider the tangential direction, as shown in Supplementary Fig. 4b. Following the previous approach, considering only heat flow propagating tangentially, we have:

$$\frac{\mathrm{d}}{\mathrm{d}\theta}\left(\frac{\mathrm{d}T}{\mathrm{d}\theta}\right) = 0. \tag{S36}$$

Integrating this equation and setting:

$$\begin{cases} T = T_1, \theta = \theta_1 \\ T = T_2, \theta = \theta_2 \end{cases}. \tag{S37}$$

we eventually obtain:

$$\frac{\mathrm{d}T}{\mathrm{d}\theta} = \frac{T_2 - T_1}{\theta_2 - \theta_1}. \tag{S38}$$

According to Fourier's law, the tangential heat flux density is:

$$q_{\mathrm{t}} = -\kappa\frac{\mathrm{d}T}{R\mathrm{d}\theta} = \kappa\frac{T_1 - T_2}{R\,(\theta_2 - \theta_1)}. \tag{S39}$$

Converting the heat flux to heat flow, we get:

$$Q_{\mathrm{t}} = \int_{R_1}^{R_2} \kappa l \frac{T_1 - T_2}{R\,(\theta_2 - \theta_1)}\mathrm{d}R = \kappa l\frac{T_1 - T_2}{(\theta_2 - \theta_1)}\ln\frac{R_2}{R_1} = \frac{T_1 - T_2}{(\theta_2 - \theta_1)\big/\left(\kappa l \ln\frac{R_2}{R_1}\right)}. \tag{S40}$$

Thus, the tangential thermal resistance is $(\theta_2 - \theta_1)\Big/\left(\kappa l \ln\frac{R_2}{R_1}\right)$.

## 4.3 Equivalent thermal resistance methods for the calculation

Next, let us analyze the equivalent radial and tangential thermal conductivities enabled by the alternately arranged materials A and B. Using parallel and series formulas, we have

$$\begin{cases} \dfrac{\frac{\ln\frac{R_2}{R_1}}{(\theta_2-\theta_1)\kappa_1 l} \times \frac{\ln\frac{R_2}{R_1}}{(\theta_3-\theta_2)\kappa_2 l}}{\frac{\ln\frac{R_2}{R_1}}{(\theta_2-\theta_1)\kappa_1 l} + \frac{\ln\frac{R_2}{R_1}}{(\theta_3-\theta_2)\kappa_2 l}} = \dfrac{\ln\frac{R_2}{R_1}}{(\theta_3 - \theta_1)\,\kappa_{\mathrm{r}} l} \\ \dfrac{\theta_2 - \theta_1}{\kappa_1 l \ln\frac{R_2}{R_1}} + \dfrac{\theta_3 - \theta_2}{\kappa_2 l \ln\frac{R_2}{R_1}} = \dfrac{\theta_3 - \theta_1}{\kappa_{\mathrm{t}} l \ln\frac{R_2}{R_1}} \end{cases} \tag{S41}$$

After rearrangement, we get:

$$\begin{cases}\kappa_{\mathrm{r}}=\dfrac{(\theta_3-\theta_2)\,\kappa_2+(\theta_2-\theta_1)\,\kappa_1}{\theta_3-\theta_1}\\ \kappa_{\mathrm{t}}=\dfrac{(\theta_3-\theta_1)\,\kappa_1\kappa_2}{(\theta_2-\theta_1)\,\kappa_2+(\theta_3-\theta_2)\,\kappa_1}\end{cases}. \tag{S42}$$

The above results are consistent with those in the literature [1].

# 5 Relationships between cooling enhancement rates and IHS power density

It can be observed that all the characteristic temperatures of the IHS, $T_{\mathrm{max}}$, $T_{\mathrm{ave}}$, and $T_{\mathrm{min}}$, can be expressed as the following form:

$$\begin{cases}T_w=A_w\dot{\phi}_{\mathrm{h}}+T_{\mathrm{f,in}}\\ T'_w=B_w\dot{\phi}_{\mathrm{h}}+T_{\mathrm{f,in}}\end{cases}, \tag{S43}$$

where $T_w$ and $T'_w$ represent the cases without and with CMTD, respectively; $w=1,2,3$ denotes the cases for $T_{\mathrm{max}}$, $T_{\mathrm{ave}}$, and $T_{\mathrm{min}}$, respectively. For $T_{\mathrm{max}}$:

$$\begin{cases}A_1=\dfrac{1}{4\kappa_{\mathrm{h}}}R_1^2+\dfrac{R_1^2}{2\kappa_{\mathrm{r}}}\ln\dfrac{R_2}{R_1}+\dfrac{R_1^2}{2hR_2}+\dfrac{\pi R_1^2 d_{\mathrm{z}}}{c\dot{m}}\\ B_1=\dfrac{1}{4\kappa_{\mathrm{h}}}\left(R_1+\dfrac{\pi R_1\kappa_{\mathrm{h}}d_{\mathrm{z}}}{c\dot{m}}\right)^2+\dfrac{R_1^2}{2\kappa_{\mathrm{r}}}\ln\dfrac{R_2}{R_1}+\dfrac{R_1^2}{2hR_2}\end{cases}. \tag{S44}$$

For $T_{\mathrm{ave}}$:

$$\begin{cases}A_2=\left(\dfrac{1}{6\kappa_{\mathrm{h}}}+\dfrac{1}{2hR_2}+\dfrac{1}{2\kappa_{\mathrm{r}}}\ln\dfrac{R_2}{R_1}+\dfrac{\pi d_{\mathrm{z}}}{c_{\mathrm{f}}\dot{m}}\right)R_1^2\\ B_2=\dfrac{2aR_1}{9\kappa_{\mathrm{h}}}+\dfrac{R_1^2}{2hR_2}+\dfrac{R_1^2}{2\kappa_{\mathrm{r}}}\ln\dfrac{R_2}{R_1}+\dfrac{(a+R_1)^2}{36\kappa_{\mathrm{h}}}\left(5+\dfrac{K\left[-\frac{4aR_1}{(R_1-a)^2}\right]}{E\left[-\frac{4aR_1}{(R_1-a)^2}\right]}\right)\end{cases}. \tag{S45}$$

For $T_{\mathrm{min}}$:

$$\begin{cases}A_3=\dfrac{R_1^2}{2\kappa_{\mathrm{r}}}\ln\dfrac{R_2}{R_1}+\dfrac{R_1^2}{2hR_2}+\dfrac{\pi R_1^2 d_{\mathrm{z}}}{c\dot{m}}\\ B_3=\dfrac{R_1^2}{2\kappa_{\mathrm{r}}}\ln\dfrac{R_2}{R_1}+\dfrac{R_1^2}{2hR_2}\end{cases}. \tag{S46}$$

Fig. 2b shows that under a significant CMTD effect, $T_{\mathrm{max}}>T'_{\mathrm{max}}$ & $T_{\mathrm{ave}}>T'_{\mathrm{ave}}$ & $T_{\mathrm{min}}>T'_{\mathrm{min}}$. Thus, $A_1>B_1$ & $A_2>B_2$ & $A_3>B_3$, which leads to $A_w>B_w$.

According to the definition of cooling enhancement rates, we have

$$\begin{cases} \eta_w = \dfrac{A_w - B_w}{A_w + T_{\mathrm{f,in}}/\dot{\phi}_{\mathrm{h}}} \\ \dfrac{\mathrm{d}\eta_w}{\mathrm{d}\dot{\phi}_{\mathrm{h}}} = \dfrac{(A_w - B_w)\, T_{\mathrm{f,in}}}{\left(A_w \dot{\phi}_{\mathrm{h}} + T_{\mathrm{f,in}}\right)^2} \end{cases} . \tag{S47}$$

Eq. (S47) indicates the increasing $\eta_w$ and decrease $\frac{\mathrm{d}\eta_w}{\mathrm{d}\dot{\phi}_{\mathrm{h}}}$ with the increasing $\dot{\phi}_{\mathrm{h}}$, which is consistent with the simulation results in the manuscript.

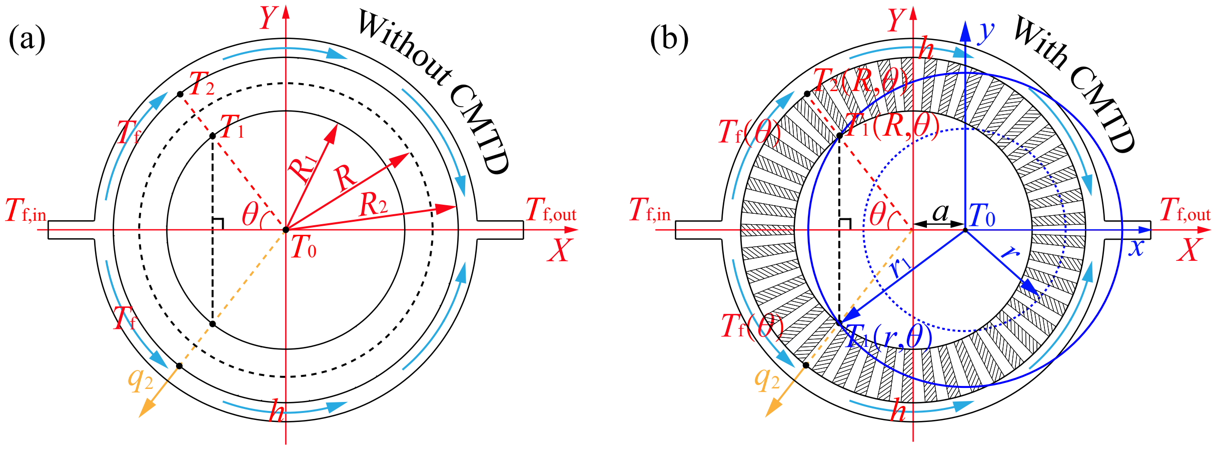


**Supplementary Fig. 1**| Used for theoretical analysis, the heat transfer model for the situation without (a) CMTD and with CMTD (b). Here, $T_0$ represents the highest temperature point of the IHS and serves as the origin of the coordinate system (a) or sub-coordinate system (b). For convenience in subsequent discussions, $T_0$ can also be denoted as the maximum temperature of the IHS ($T_{\max}$).

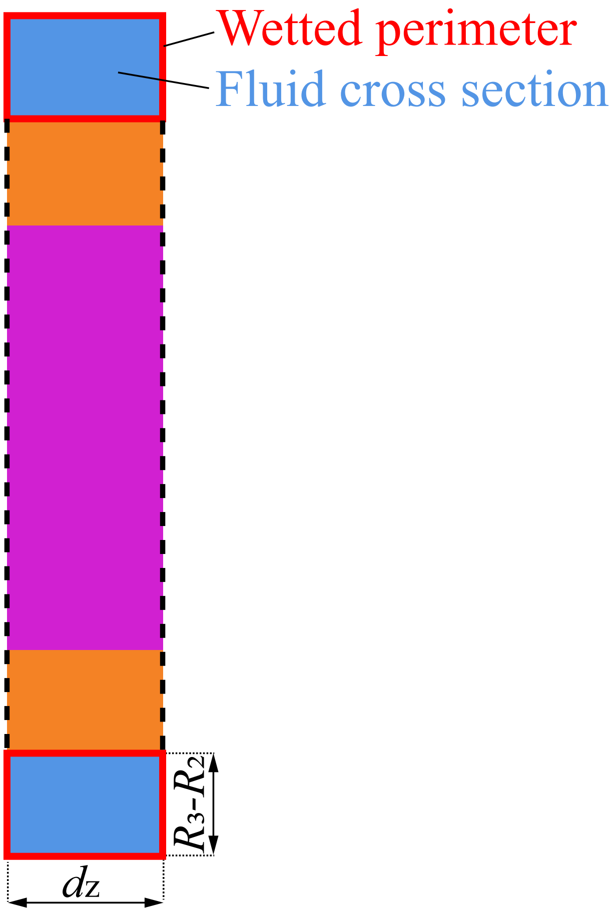


**Supplementary Fig. 2**| Cross-sectional view of the heat transfer model illustrated in Fig. 1e.

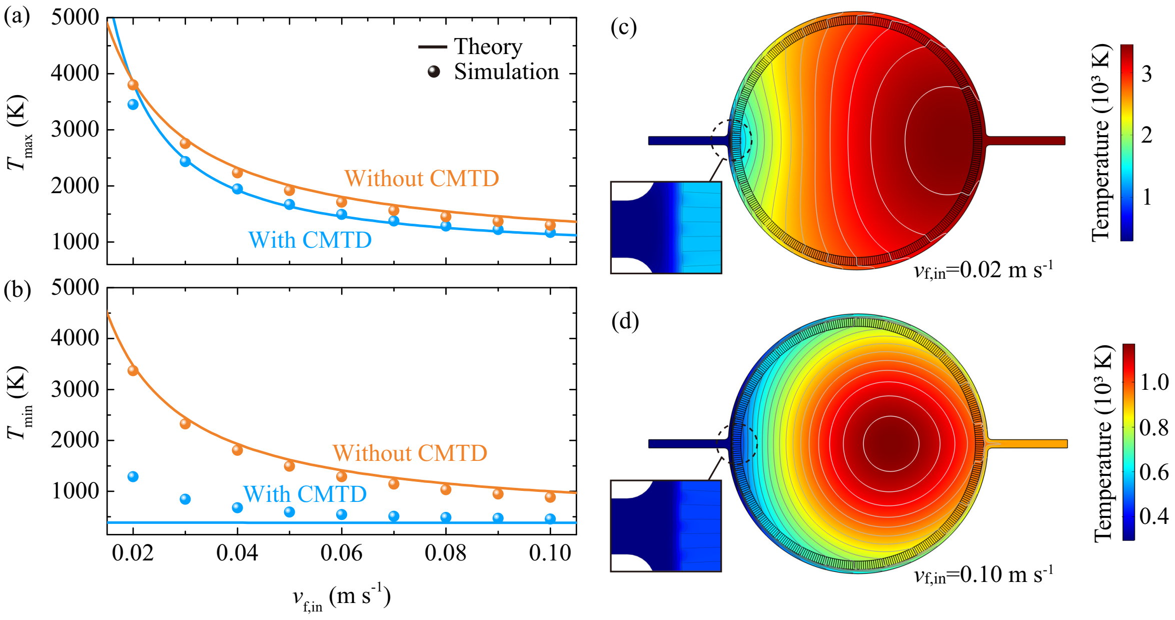


**Supplementary Fig. 3**| (a,b) The maximum temperature $T_{\max}$ (a) and the minimum temperature $T_{\min}$ (b) of the IHS versus the inlet fluid velocity $v_{\mathrm{f,in}}$. (c,d) Temperature distributions of the heat transfer model under different $v_{\mathrm{f,in}} = 0.02\,\mathrm{m\,s^{-1}}$ (c) and $v_{\mathrm{f,in}} = 0.10\,\mathrm{m\,s^{-1}}$ (d), respectively. Notably, at low flow velocities ($v_{\mathrm{in}} < 0.04\,\mathrm{m\,s^{-1}}$), a deviation is observed in the minimum temperature $T_{\min}$ of the IHS. This discrepancy arises from the assumption $T_{\mathrm{f}}(\theta)|_{\theta=0} \rightarrow T_{\mathrm{f,in}}$, leading to errors at low flow velocities, as depicted in (d).

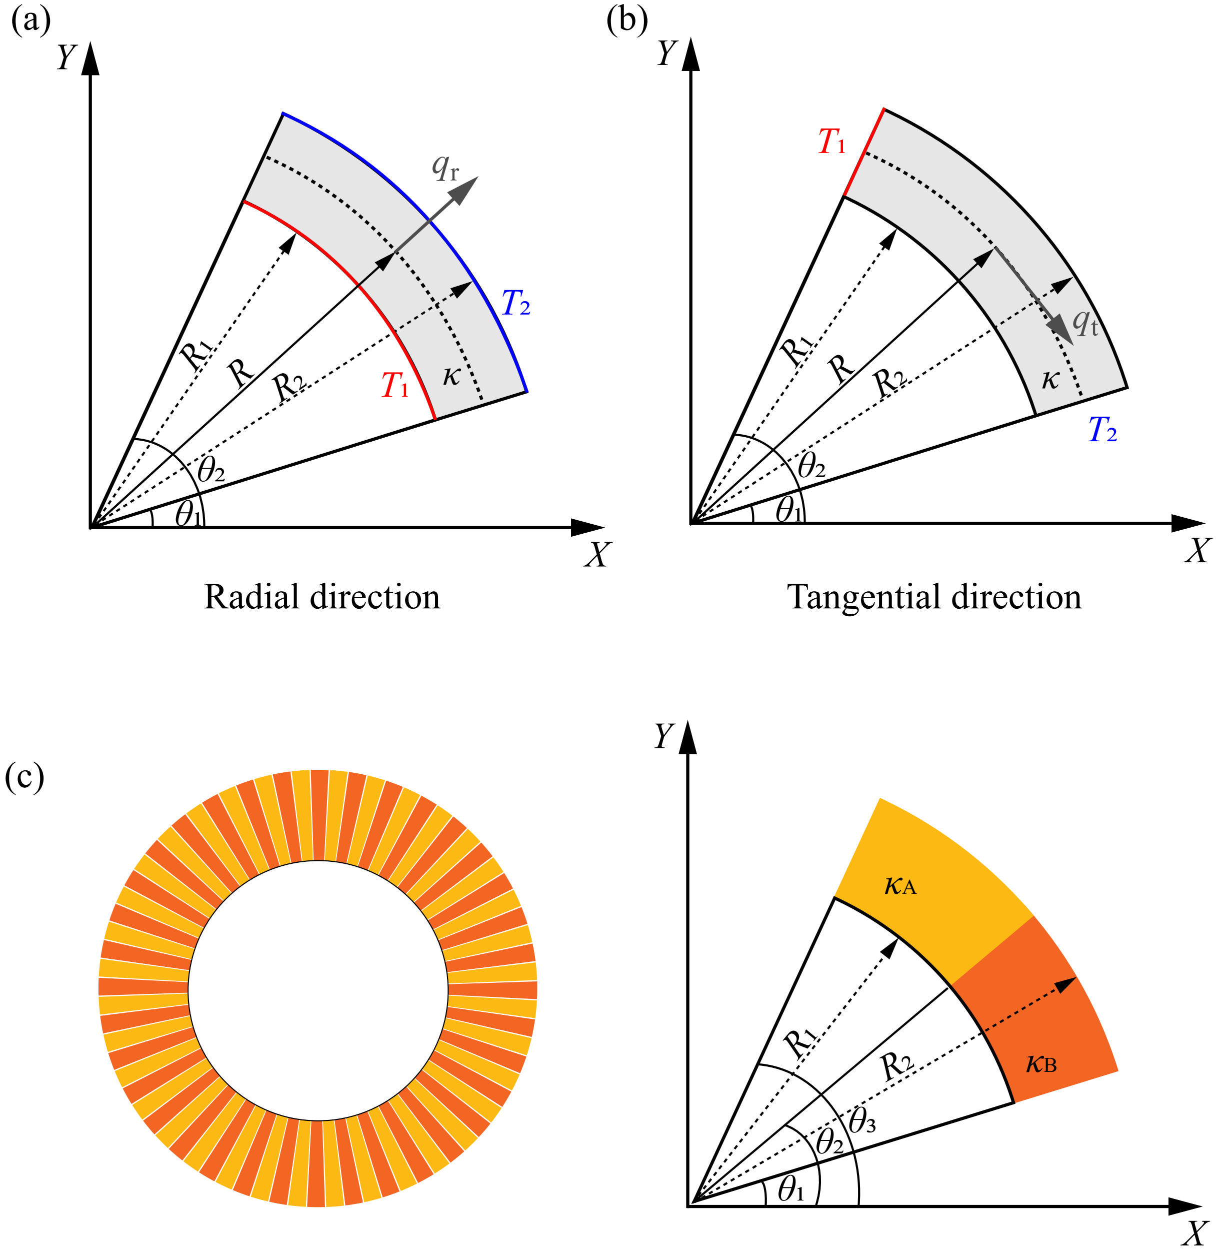


**Supplementary Fig. 4**| (a,b) Used for theoretical analysis, the radial and tangential heat transfer model for obtaining the thermal resistance. (c) Combinations of materials A and B for obtaining the analytical expressions of $\kappa_r$ and $\kappa_t$, with thermal conductivities of $\kappa_A$ and $\kappa_B$, respectively.

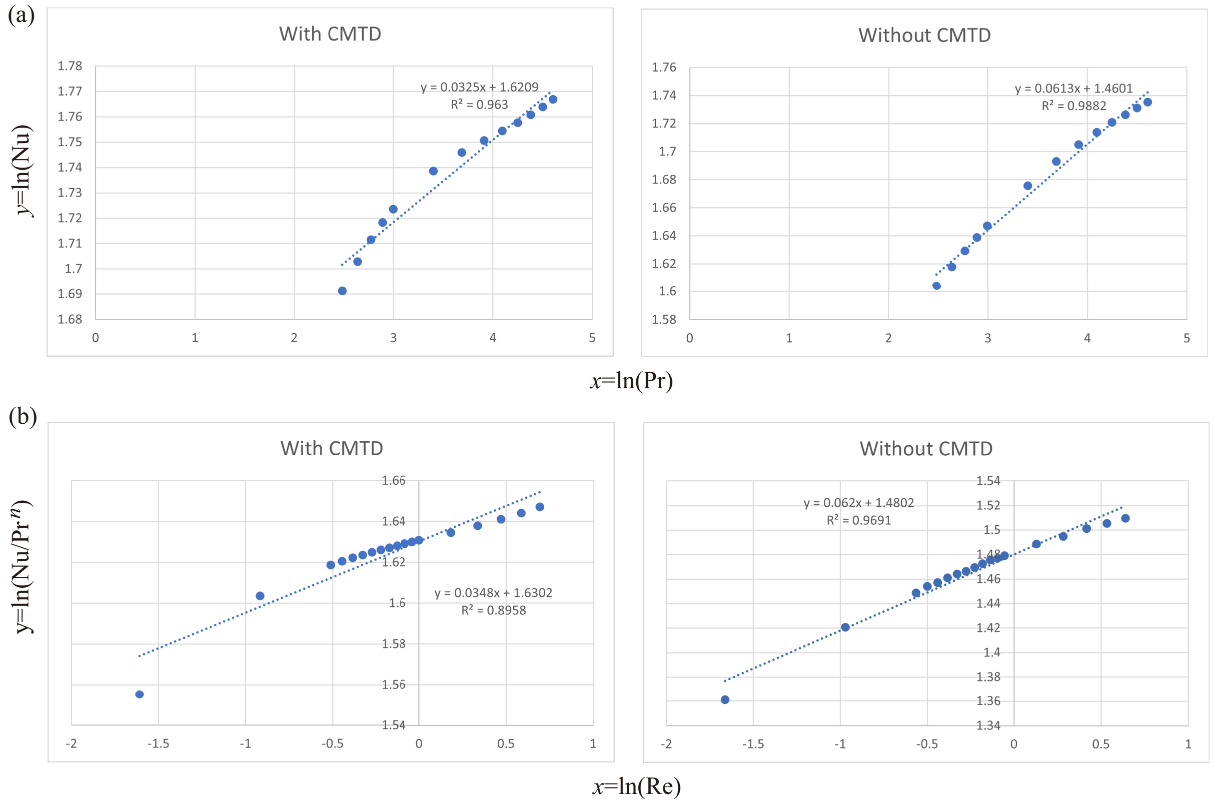


**Supplementary Fig. 5**| (a) The relationships between $\ln(\mathrm{Nu})$ and $\ln(\mathrm{Pr})$ under the cases with and without CMTD. (b) The relationships between $\ln\left(\mathrm{Nu}/\mathrm{Pr}^{n}\right)$ and $\ln(\mathrm{Re})$ under the cases with and without CMTD. See more details in Supplementary Tables 1 and 2.

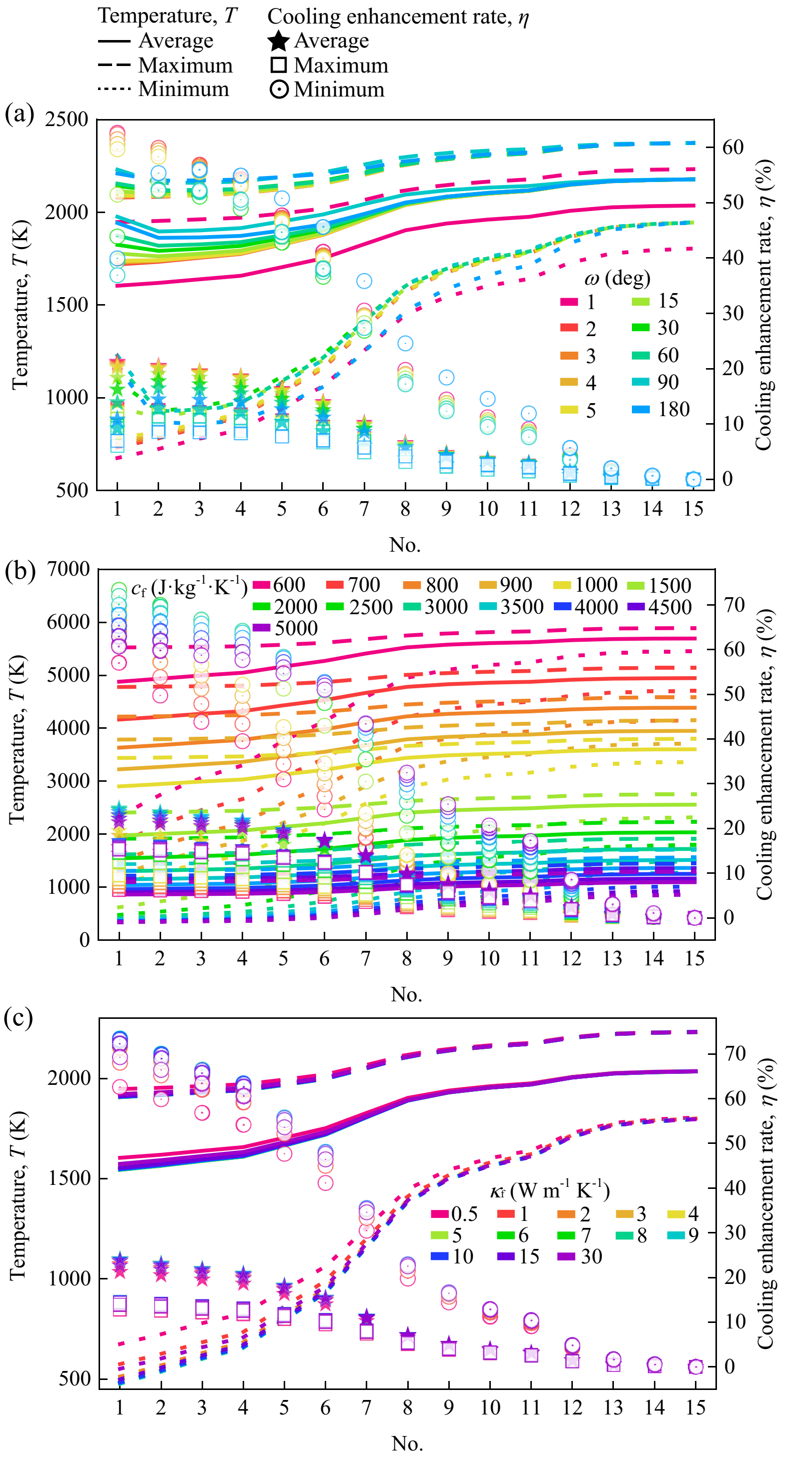


**Supplementary Fig. 6**| (a) $T_{\max}$, $T_{\text{ave}}$, $T_{\min}$, $\eta_{\max}$, $\eta_{\text{ave}}$, and $\eta_{\min}$ versus different anisotropic degrees of the thermal conductivity of the package structure under different $\omega$ (a), $c_{\text{f}}$ (b), and $\kappa_{\text{f}}$ (c). See operating conditions in Supplementary Tables 4 and 5. Notes: Subgraph (a) indicates that a smaller $\omega$ results in higher cooling enhancement rates, which can be attributed to the improved construction of low $\kappa_{\text{t}}$ and high $\kappa_{\text{r}}$. Therefore, we adopted $\omega = 1^{\circ}$ in the remaining simulations in this work.

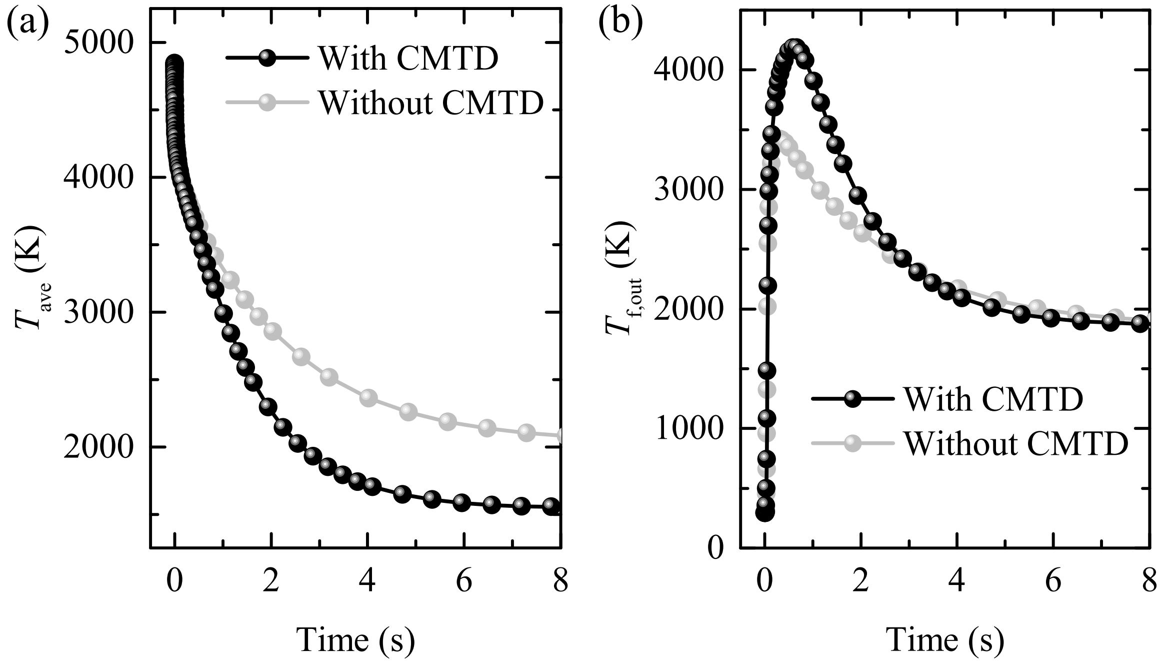


**Supplementary Fig. 7**| Transient cooling enhancement characteristics under $\kappa_{\rm f} = 5\ {\rm W\ m^{-1}\ K^{-1}}$ when $T_{\rm h,in} = 5000\ {\rm K}$. (a) Relationship between the average temperature of the IHS ($T_{\rm ave}$) and time under the transient cooling process with and without CMTD. (b) Relationship between the outlet temperature of the cooling fluid ($T_{\rm f,out}$) and time. Note that the remaining operating conditions in this simulation are the same as Fig. 8a,c ($T_{\rm h,in} = 5000$ K).

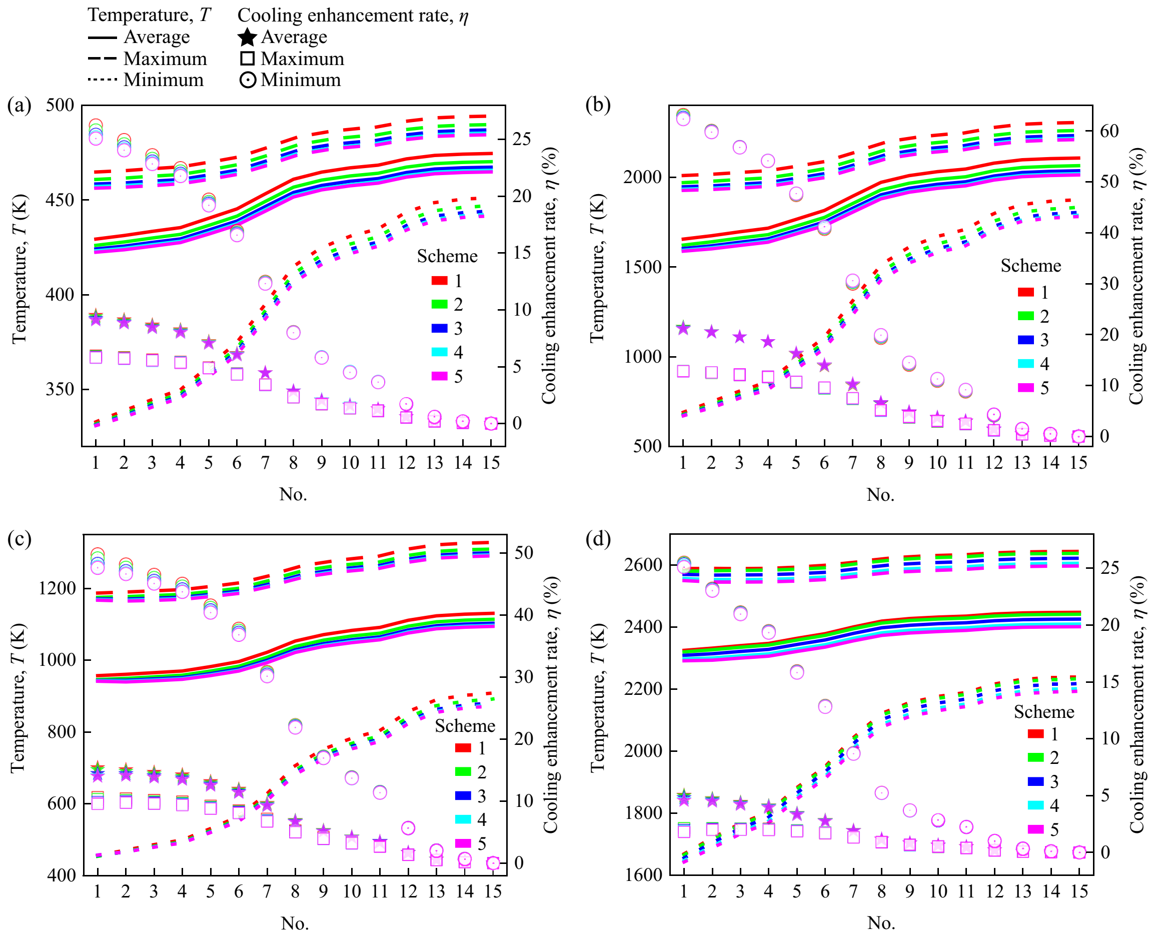


**Supplementary Fig. 8**| Influence of grid schemes on the IHS temperatures ($T_{\max}$, $T_{\text{ave}}$, and $T_{\min}$) and cooling enhancement rates ($\eta_{\max}$, $\eta_{\text{ave}}$, and $\eta_{\min}$). (a), (b), (c), and (d) correspond to cases 1, 2, 3, and 4 in Supplementary Table 8, respectively.

**Supplementary Table 1**| Data for calculating convective heat transfer correlations under different $c_\mathrm{f}$. Here, the remaining fluidic parameters were: $\kappa_\mathrm{f} = 0.5$ W m$^{-1}$ K$^{-1}$, $\rho_\mathrm{f} = 1000$ kg m$^{-3}$, $\mu = 0.01$ Pa s, $\gamma = 1$, $v_\mathrm{f,in} = 0.04$ m s$^{-1}$, $p_\mathrm{out} = 101325$ Pa, and $T_\mathrm{f,in} = 293.15$ K. The structural parameters were: $R_1 = 2.8$ mm, $R_2 = 3.0$ mm, $R_3 = 3.1$ mm, $D = 0.2$ mm, and $\omega = 1°$. The IHS parameters was: $\kappa_\mathrm{h} = 5$ W m$^{-1}$ K$^{-1}$. For the cases with CMTD: $\kappa_\mathrm{A} = 4000$ W m$^{-1}$ K$^{-1}$ and $\kappa_\mathrm{B} = 1$ W m$^{-1}$ K$^{-1}$; for the cases without CMTD: $\kappa_\mathrm{A} = \kappa_\mathrm{B} = 4000$ W m$^{-1}$ K$^{-1}$.

| $c_\mathrm{f}$ (J kg$^{-1}$ K$^{-1}$) | CMTD (With or without) | $\langle T_\mathrm{f} \rangle$ (K) | $\langle T_\mathrm{p,o} \rangle$ (K) | $h_\mathrm{t}$ (W m$^{-2}$ K$^{-1}$) | Nu | Pr | ln Nu | ln Pr |
|---|---|---|---|---|---|---|---|---|
| 600 | With | 4578.89032 | 4675.21705 | 13564.94384 | 5.42598 | 12.00000 | 1.69120 | 2.48491 |
| | Without | 5391.68543 | 5496.77816 | 12433.46433 | 4.97339 | 12.00000 | 1.60410 | 2.48491 |
| 700 | With | 3870.00631 | 3965.21589 | 13724.10828 | 5.48964 | 14.00000 | 1.70286 | 2.63906 |
| | Without | 4647.72578 | 4751.38668 | 12605.20276 | 5.04208 | 14.00000 | 1.61782 | 2.63906 |
| 800 | With | 3346.39103 | 3440.77223 | 13844.56510 | 5.53783 | 16.00000 | 1.71160 | 2.77259 |
| | Without | 4088.35081 | 4190.83545 | 12749.87814 | 5.09995 | 16.00000 | 1.62923 | 2.77259 |
| 900 | With | 2945.68593 | 3039.43571 | 13937.81114 | 5.57512 | 18.00000 | 1.71831 | 2.89037 |
| | Without | 3653.15959 | 3754.66088 | 12873.39988 | 5.14936 | 18.00000 | 1.63887 | 2.89037 |
| 1000 | With | 2630.45497 | 2723.71146 | 14011.53587 | 5.60461 | 20.00000 | 1.72359 | 2.99573 |
| | Without | 3306.42841 | 3407.09929 | 12979.58904 | 5.19184 | 20.00000 | 1.64709 | 2.99573 |
| 1500 | With | 1727.44338 | 1819.30476 | 14224.33076 | 5.68973 | 30.00000 | 1.73866 | 3.40120 |
| | Without | 2264.55406 | 2362.38165 | 13356.83187 | 5.34273 | 30.00000 | 1.67574 | 3.40120 |
| 2000 | With | 1310.77887 | 1401.97232 | 14328.51387 | 5.73141 | 40.00000 | 1.74596 | 3.68888 |
| | Without | 1744.03133 | 1840.16604 | 13592.03776 | 5.43682 | 40.00000 | 1.69319 | 3.68888 |
| 2500 | With | 1076.37579 | 1167.13697 | 14396.75603 | 5.75870 | 50.00000 | 1.75071 | 3.91202 |
| | Without | 1432.04984 | 1527.04086 | 13755.68669 | 5.50227 | 50.00000 | 1.70516 | 3.91202 |
| 3000 | With | 928.00985 | 1018.43323 | 14450.53942 | 5.78022 | 60.00000 | 1.75444 | 4.09434 |
| | Without | 1224.92042 | 1319.08088 | 13877.01993 | 5.55081 | 60.00000 | 1.71394 | 4.09434 |
| 3500 | With | 826.18904 | 916.31397 | 14498.39436 | 5.79936 | 70.00000 | 1.75775 | 4.24850 |
| | Without | 1077.39225 | 1170.90977 | 13972.42627 | 5.58897 | 70.00000 | 1.72080 | 4.24850 |
| 4000 | With | 752.23582 | 842.0791 | 14543.84413 | 5.81754 | 80.00000 | 1.76088 | 4.38203 |
| | Without | 967.22111 | 1060.21509 | 14051.09006 | 5.62044 | 80.00000 | 1.72641 | 4.38203 |
| 4500 | With | 696.29822 | 785.86962 | 14587.99069 | 5.83520 | 90.00000 | 1.76391 | 4.49981 |
| | Without | 882.03044 | 974.58128 | 14118.36667 | 5.64735 | 90.00000 | 1.73119 | 4.49981 |
| 5000 | With | 652.42962 | 741.7336 | 14631.67252 | 5.85267 | 100.00000 | 1.76690 | 4.60517 |
| | Without | 814.37341 | 906.53678 | 14177.72163 | 5.67109 | 100.00000 | 1.73538 | 4.60517 |

**Supplementary Table 2**| Data for calculating convective heat transfer correlations under different $v_{\mathrm{f,in}}$ are provided below. Here, $c_{\mathrm{f}} = 2000$ J kg$^{-1}$ K$^{-1}$. The remaining parameters are the same as those of Supplementary Table 1. Notes: For the cases with CMTD, $n = 0.0325$; for the cases without CMTD, $n = 0.0613$ (See the details in Supplementary Fig. 5).

| $v_{\mathrm{f,in}}$ (m s$^{-1}$) | CMTD (With or without) | $\langle T_{\mathrm{f}} \rangle$ (K) | $\langle T_{\mathrm{p,o}} \rangle$ (K) | $h_{\mathrm{t}}$ (W m$^{-2}$ K$^{-1}$) | Nu | Re | ln Re | ln Nu/Pr$^{n}$ |
|---|---|---|---|---|---|---|---|---|
| 0.010 | With | 5585.02848 | 5682.92226 | 13347.80013 | 5.33912 | 0.20000 | -1.60944 | 1.55517 |
| | Without | 6435.60095 | 6542.52122 | 12220.94433 | 4.88838 | 0.20000 | -1.60944 | 1.36073 |
| 0.020 | With | 2630.40316 | 2723.66600 | 14010.58194 | 5.60423 | 0.40000 | -0.91629 | 1.60363 |
| | Without | 3306.34705 | 3407.03635 | 12977.21468 | 5.19089 | 0.40000 | -0.91629 | 1.42078 |
| 0.030 | With | 1727.42867 | 1819.29249 | 14223.95421 | 5.68958 | 0.60000 | -0.51083 | 1.61875 |
| | Without | 2264.52720 | 2362.36364 | 13355.62329 | 5.34225 | 0.60000 | -0.51083 | 1.44952 |
| 0.032 | With | 1620.73100 | 1712.42831 | 14249.78220 | 5.69991 | 0.64000 | -0.44629 | 1.62056 |
| | Without | 2133.89625 | 2231.32602 | 13411.36856 | 5.36455 | 0.64000 | -0.44629 | 1.45368 |
| 0.034 | With | 1527.65563 | 1619.20534 | 14272.75488 | 5.70910 | 0.68000 | -0.38566 | 1.62217 |
| | Without | 2019.39687 | 2116.46083 | 13461.91476 | 5.38477 | 0.68000 | -0.38566 | 1.45745 |
| 0.036 | With | 1446.41922 | 1537.83845 | 14293.12819 | 5.71725 | 0.72000 | -0.32850 | 1.62360 |
| | Without | 1917.58102 | 2014.31017 | 13508.50959 | 5.40340 | 0.72000 | -0.32850 | 1.46090 |
| 0.038 | With | 1374.42618 | 1465.72669 | 14311.71233 | 5.72468 | 0.76000 | -0.27444 | 1.62490 |
| | Without | 1825.91411 | 1922.33213 | 13552.09978 | 5.42084 | 0.76000 | -0.27444 | 1.46412 |
| 0.040 | With | 1310.77887 | 1401.97232 | 14328.51387 | 5.73141 | 0.80000 | -0.22314 | 1.62607 |
| | Without | 1744.03133 | 1840.16604 | 13592.03776 | 5.43682 | 0.80000 | -0.22314 | 1.46707 |
| 0.042 | With | 1253.88726 | 1344.98219 | 14344.01053 | 5.73760 | 0.84000 | -0.17435 | 1.62715 |
| | Without | 1669.92721 | 1765.79942 | 13629.25327 | 5.45170 | 0.84000 | -0.17435 | 1.46980 |
| 0.044 | With | 1202.56233 | 1293.56492 | 14358.56578 | 5.74343 | 0.88000 | -0.12783 | 1.62817 |
| | Without | 1602.06364 | 1697.68856 | 13664.50022 | 5.46580 | 0.88000 | -0.12783 | 1.47238 |
| 0.046 | With | 1156.46195 | 1247.37915 | 14372.05136 | 5.74882 | 0.92000 | -0.08338 | 1.62911 |
| | Without | 1540.65151 | 1636.04953 | 13696.99969 | 5.47880 | 0.92000 | -0.08338 | 1.47476 |
| 0.048 | With | 1114.64729 | 1205.48402 | 14384.78322 | 5.75391 | 0.96000 | -0.04082 | 1.62999 |
| | Without | 1484.34665 | 1579.53251 | 13727.52974 | 5.49101 | 0.96000 | -0.04082 | 1.47698 |
| 0.050 | With | 1076.38442 | 1167.14390 | 14397.02737 | 5.75881 | 1.00000 | 0.00000 | 1.63084 |

**Supplementary Table 2 continued from previous page**

| | | | | | | | | |
|---|---|---|---|---|---|---|---|---|
| | Without | 1432.07430 | 1527.05786 | 13756.76712 | 5.50271 | 1.00000 | 0.00000 | 1.47911 |
| 0.060 | With | 928.02237 | 1018.44269 | 14451.02909 | 5.78041 | 1.20000 | 0.18232 | 1.63459 |
| | Without | 1224.95797 | 1319.10475 | 13879.03775 | 5.55162 | 1.20000 | 0.18232 | 1.48796 |
| 0.070 | With | 826.20494 | 916.32579 | 14499.04936 | 5.79962 | 1.40000 | 0.33647 | 1.63790 |
| | Without | 1077.43945 | 1170.93815 | 13975.23939 | 5.59010 | 1.40000 | 0.33647 | 1.49487 |
| 0.080 | With | 752.25561 | 842.09402 | 14544.63336 | 5.81785 | 1.60000 | 0.47000 | 1.64104 |
| | Without | 967.27711 | 1060.24798 | 14054.58093 | 5.62183 | 1.60000 | 0.47000 | 1.50053 |
| 0.090 | With | 696.31559 | 785.88158 | 14588.87106 | 5.83555 | 1.80000 | 0.58779 | 1.64408 |
| | Without | 882.09540 | 974.61979 | 14122.40252 | 5.64896 | 1.80000 | 0.58779 | 1.50534 |
| 0.100 | With | 652.45121 | 741.74944 | 14632.61548 | 5.85305 | 2.00000 | 0.69315 | 1.64707 |
| | Without | 814.44853 | 906.58277 | 14182.20490 | 5.67288 | 2.00000 | 0.69315 | 1.50957 |

**Supplementary Table 3**| Combinations of materials A and B for CMTD under different anisotropic degrees of thermal conductivity of the package structure.

| No. | 1 | 2 | 3 | 4 | 5 | 6 | 7 | 8 |
|---|---|---|---|---|---|---|---|---|
| $\kappa_A$ ($W\ m^{-1}\ K^{-1}$) | 4000 | 4000 | 4000 | 4000 | 4000 | 4000 | 4000 | 4000 |
| $\kappa_B$ ($W\ m^{-1}\ K^{-1}$) | 1 | 5 | 10 | 15 | 30 | 50 | 100 | 200 |
| No. | 9 | 10 | 11 | 12 | 13 | 14 | 15 | / |
| $\kappa_A$ ($W\ m^{-1}\ K^{-1}$) | 4000 | 4000 | 4000 | 4000 | 4000 | 4000 | 4000 | / |
| $\kappa_B$ ($W\ m^{-1}\ K^{-1}$) | 300 | 400 | 500 | 1000 | 2000 | 3000 | 4000 | / |

**Supplementary Table 4**| Operating conditions for studying the structural parameters on the CMTD effect (Fig. 4). The remaining structural parameters were: $D = 0.2$ mm and $L = 5$ mm. The fluidic parameters were: $\kappa_\mathrm{f} = 0.5$ W m$^{-1}$ K$^{-1}$, $\rho_\mathrm{f} = 1000$ kg m$^{-3}$, $c_\mathrm{f} = 2000$ J kg$^{-1}$ K$^{-1}$, $\mu = 0.01$ Pa s, $v_\mathrm{f,in} = 0.04$ m s$^{-1}$, $p_\mathrm{out} = 101325$ Pa, and $T_\mathrm{f,in} = 293.15$ K. The IHS parameters were: $\dot{\phi}_\mathrm{h} = 1 \times 10^9$ W m$^{-3}$ and $\kappa_\mathrm{h} = 5$ W m$^{-1}$ K$^{-1}$.

| Case | $R_1$ (mm) | $R_2$ (mm) | $R_3$ (mm) | $\omega$ (deg) |
|---|---|---|---|---|
| Fig. 4a (upper subgraph) | 2.8 | 3.0 | 3.1, 3.2, 3.3, 3.4, 3.5, 3.6, 3.7, 3.8, 3.9, 4.0 | 1 |
| Fig. 4a (lower subgraph) | 2.0, 2.1, 2.2 2.3, 2.4, 2.5, 2.6, 2.7, 2.8, 2.9 | 3.0 | 3.1 | 1 |
| Supplementary Fig. 6a | 2.8 | 3.0 | 3.1 | 1, 2, 3, 4, 5, 15, 30, 60, 90, 180 |

**Supplementary Table 5**| Operating conditions for studying the fluidic parameters on the CMTD effect (Fig. 5). Here, the structural parameters were: $R_1 = 2.8$ mm, $R_2 = 3.0$ mm, $R_3 = 3.1$ mm, $D = 0.2$ mm, $L = 5$ mm, and $\omega = 1°$. The IHS parameters were: $\dot{\phi}_\mathrm{h} = 1 \times 10^9$ W m$^{-3}$ and $\kappa_\mathrm{h} = 5$ W m$^{-1}$ K$^{-1}$. The remaining fluidic parameters were: $p_\mathrm{out} = 101325$ Pa and $T_\mathrm{f,in} = 293.15$ K.

| Case | $\kappa_\mathrm{f}$ (W m$^{-1}$ K$^{-1}$) | $\rho_\mathrm{f}$ (kg m$^{-3}$) | $c_\mathrm{f}$ (J kg$^{-1}$ K$^{-1}$) | $\mu$ (Pa s) | $v_\mathrm{f,in}$ (m s$^{-1}$) |
|---|---|---|---|---|---|
| Fig. 5a (upper subgraph) | 0.5 | 1000 | 2000 | 0.01 | 0.01, 0.02, 0.03, 0.04, 0.05, 0.06, 0.07, 0.08, 0.09, 0.10 |
| Fig. 5a (lower subgraph) | 5 | 200, 300, 400, 500, 600, 700, 800, 900, 1000, 2000, 3000, 4000, 5000 | 2000 | 0.01 | 0.04 |
| Supplementary Fig. 6b | 5 | 1000 | 600, 700, 800, 900, 1000, 1500, 2000, 2500, 3000, 3500, 4000, 4500 | 0.01 | 0.04 |
| Supplementary Fig. 6c | 0.5, 1, 2, 3, 4, 5, 6, 7, 8, 9, 10, 15, 30 | 1000 | 2000 | 0.01 | 0.04 |

**Supplementary Table 6**| Operating conditions for studying the IHS parameters on the CMTD effect (Fig. 6). Here, the fluidic parameters were: $\kappa_{\mathrm{f}} = 0.5\ \mathrm{W\ m^{-1}\ K^{-1}}$, $\rho_{\mathrm{f}} = 1000\ \mathrm{kg\ m^{-3}}$, $c_{\mathrm{f}} = 2000\ \mathrm{J\ kg^{-1}\ K^{-1}}$, $\mu = 0.01\ \mathrm{Pa\,s}$, $v_{\mathrm{f,in}} = 0.04\ \mathrm{m\,s^{-1}}$, $p_{\mathrm{out}} = 101325\ \mathrm{Pa}$, and $T_{\mathrm{f,in}} = 293.15\ \mathrm{K}$. The structural parameters were: $R_1 = 2.8\ \mathrm{mm}$, $R_2 = 3.0\ \mathrm{mm}$, $R_3 = 3.1\ \mathrm{mm}$, $D = 0.2\ \mathrm{mm}$, $L = 5\ \mathrm{mm}$, and $\omega = 1°$.

| Case | $\kappa_{\mathrm{h}}$ ($\mathrm{W\ m^{-1}\ K^{-1}}$) | $\dot{\phi}_{\mathrm{h}}$ ($\times 10^9\ \mathrm{W\ m^{-3}}$) |
|---|---|---|
| Fig. 6a (upper subgraph) | 1, 5, 10, 15, 30, 50, 100, 200, 300, 400, 500, 1000, 2000, 3000, 4000 | 1 |
| Fig. 6b (lower subgraph) | 1 | 0.1, 0.2, 0.3, 0.4, 0.5, 0.6, 0.7, 0.8, 0.9, 1 |

**Supplementary Table 7**| Cases for grid independence test.

| Case | $v_{\mathrm{f,in}}$ $(\mathrm{m\,s^{-1}})$ | $R_3$ (mm) | $\dot{\phi}_\mathrm{h}$ $(\times 10^9\ \mathrm{W\,m^{-3}})$ |
|---|---|---|---|
| 1 | 0.04 | 3.1 | 0.1 |
| 2 | 0.04 | 3.1 | 1.0 |
| 3 | 0.10 | 3.1 | 1.0 |
| 4 | 0.04 | 4.0 | 1.0 |

**Supplementary Table 8**| Grid independence test for the heat transfer model in Fig. 1e.

| Case | Scheme | Grid number | $T_{\mathrm{f,out}}$ (K) Simulation results | $T_{\mathrm{f,out}}$ (K) Theoretical results | Relative error (%) |
|---|---|---|---|---|---|
| 1 | 1 | 31466 | 457.08-457.13 | 447.088 | 2.2 |
| | 2 | 41390 | 452.72-452.81 | | 1.3 |
| | 3 | 349052 | 449.78-449.91 | | 0.6 |
| | 4 | 1396080 | 447.99-448.26 | | 0.2-0.3 |
| | 5 | 5584832 | 446.81-447.43 | | -0.1-0.1 |
| 2 | 1 | 31466 | 1933.0-1933.4 | 1832.530 | 5.5 |
| | 2 | 41390 | 1889.7-1890.1 | | 3.1 |
| | 3 | 349052 | 1860.6-1861.4 | | 1.5-1.6 |
| | 4 | 1396208 | 1844.5-1845.6 | | 0.7 |
| | 5 | 5584832 | 1836.1-1838.3 | | 0.2-0.3 |
| 3 | 1 | 31466 | 948.99-949.22 | 908.902 | 4.4 |
| | 2 | 41390 | 931.61-931.89 | | 2.5 |
| | 3 | 349052 | 919.92-920.37 | | 1.2-1.3 |
| | 4 | 1396208 | 913.24-914.00 | | 0.5-0.6 |
| | 5 | 5584320 | 908.59-910.88 | | 0-0.2 |
| 4 | 1 | 35916 | 1902.8-1903.3 | 1832.530 | 3.8-3.9 |
| | 2 | 49562 | 1892.9-1893.4 | | 3.3 |
| | 3 | 374456 | 1871.2-1872.0 | | 2.1-2.2 |
| | 4 | 1497824 | 1849.5-1851.0 | | 0.9-1.0 |
| | 5 | 5991296 | 1836.9-1839.6 | | 0.2-0.4 |

# References

[1] Wudi Wang. *Numerical Simulation of Thermal Cloak and Heat Flux Control*. Harbin Institute of Technology, 2018.
